# Supplementary material for: Intuitionistic Fuzzy Broad Learning System: Enhancing Robustness Against Noise and Outliers
Source: arXiv:2307.08713 source file (2024-05-11)
Supplement: Supplementary file 2 [file IF_BLS_supplementary_file.pdf]

# Supplementary Material for the Manuscript “Intuitionistic Fuzzy Broad Learning System: Enhancing Robustness Against Noise and Outliers”

M. Sajid, A.K. Malik, M. Tanveer, for the Alzheimer’s Disease Neuroimaging Initiative

## S.I. KERNEL TECHNIQUE USED FOR FINDING RADIUS IN ASSIGNING INTUITIONISTIC FUZZY SCORE

The Kernel technique is explored here.

**Theorem S.I.1.** [1]: Let  $\mathcal{K}(x_r, x_l) = \psi(x_r) \cdot \psi(x_l)$  be a Kernel function, where  $\cdot$  is the standard inner product. Then, the norm  $\|\cdot\|$  is calculated as:

$$\|\psi(x_r) - \psi(x_l)\| = \sqrt{\mathcal{K}(x_r, x_r) + \mathcal{K}(x_l, x_l) - 2\mathcal{K}(x_r, x_l)}. \quad (1)$$

*Proof.*

$$\begin{aligned} \|\psi(x_r) - \psi(x_l)\|^2 &= (\psi(x_r) - \psi(x_l)) \cdot (\psi(x_r) - \psi(x_l)) \\ &= \psi(x_r) \cdot \psi(x_r) + \psi(x_l) \cdot \psi(x_l) - 2\psi(x_r) \cdot \psi(x_l) \\ &= \mathcal{K}(x_r, x_r) + \mathcal{K}(x_l, x_l) - 2\mathcal{K}(x_r, x_l). \end{aligned}$$

□

**Theorem S.I.2.** [1]: The radii  $R_{pos}$  and  $R_{neg}$  are calculated as:

$$R_{pos} = \max_{t_r=+1} \sqrt{\mathcal{K}(x_r, x_r) + \frac{1}{N_{pos}^2} \sum_{t_i=+1} \sum_{t_j=+1} \mathcal{K}(x_i, x_j) - \frac{2}{N_{pos}} \sum_{t_l=+1} \mathcal{K}(x_r, x_l)} \quad (2)$$

$$R_{neg} = \max_{t_r=-1} \sqrt{\mathcal{K}(x_r, x_r) + \frac{1}{N_{neg}^2} \sum_{t_i=-1} \sum_{t_j=-1} \mathcal{K}(x_i, x_j) - \frac{2}{N_{neg}} \sum_{t_l=-1} \mathcal{K}(x_r, x_l)}. \quad (3)$$

*Proof.*

$$\begin{aligned} R_{pos} &= \max_{t_r=+1} \|\psi(x_r) - C_{pos}\| \\ &= \max_{t_r=+1} \sqrt{(\psi(x_r) - C_{pos}) \cdot (\psi(x_r) - C_{pos})} \\ &= \max_{t_r=+1} \sqrt{\psi(x_r) \cdot \psi(x_r) + C_{pos} \cdot C_{pos} - 2\psi(x_r) \cdot C_{pos}} \\ &= \max_{t_r=+1} \sqrt{\mathcal{K}(x_r, x_l) + \left( \frac{1}{N_{pos}} \sum_{t_i=+1} \psi(x_i) \right) \left( \frac{1}{N_{pos}} \sum_{t_j=+1} \psi(x_j) \right) - 2\psi(x_i) \left( \frac{1}{N_{pos}} \sum_{t_j=+1} \psi(x_j) \right)} \\ &= \max_{t_r=+1} \sqrt{\mathcal{K}(x_r, x_r) + \frac{1}{N_{pos}^2} \sum_{t_i=+1} \sum_{t_j=+1} \mathcal{K}(x_i, x_j) - \frac{2}{N_{pos}} \sum_{t_l=+1} \mathcal{K}(x_r, x_l)}. \end{aligned}$$

Similarly, the radius  $R_{neg}$  can be calculated.

□

## S.II. DATASETS SELECTED FOR EVALUATION ON UCI DATASETS WITH GAUSSIAN NOISE

We have chosen 5 diverse UCI datasets for our comparative analysis to evaluate the proposed F-BLS and IF-BLS models

in the presence of Gaussian noise. These datasets include breast\_cancer, conn\_bench\_sonar\_mines\_rocks, hill\_valley, pittsburg\_bridges\_T\_OR\_D, and tic\_tac\_toe, each representing a different domain. In order to ensure fairness in evaluating the models, we have selected 3 datasets where none of the proposed F-BLS and IF-BLS models achieve the highest

Table S.I  
HYPERPARAMETERS' DESCRIPTION AND RANGE FOR THE BASELINE AND PROPOSED MODELS.

| Models    | Parameters' description                                                                                                                                                                            | Parameters' Range                                                                                                                           |
|-----------|----------------------------------------------------------------------------------------------------------------------------------------------------------------------------------------------------|---------------------------------------------------------------------------------------------------------------------------------------------|
| BLS       | $C$ : Regularization parameter<br>$m$ : Number of feature groups<br>$p$ : Number of feature nodes in each groups<br>$q$ : Number of enhancement nodes                                              | $C = [10^{-6}, 10^{-4}, \dots, 10^6]$<br>$m = 1 : 2 : 21$<br>$p = 5 : 5 : 50$<br>$q = 5 : 10 : 105$                                         |
| ELM       | $C$ : Regularization parameter<br>$h_l$ : Number of hidden nodes                                                                                                                                   | $C = [10^{-6}, 10^{-4}, \dots, 10^6]$<br>$h_l = 5 : 10 : 205$                                                                               |
| NeuroFBLS | $C$ : Regularization parameter<br>$N_{fg}$ : Number of fuzzy groups<br>$N_{fn}$ : Number of fuzzy nodes in each groups<br>$q$ : Number of enhancement nodes                                        | $C = [10^{-6}, 10^{-4}, \dots, 10^6]$<br>$N_{fg} = 1 : 2 : 21$<br>$N_{fn} = 5 : 5 : 50$<br>$q = 5 : 10 : 105$                               |
| IF-TSVM   | $C_1$ : Regularization parameter for the positive class<br>$C_2$ : Regularization parameter for the negative class<br>$\mu$ : Intuitionistic fuzzy Kernel parameter                                | $C_1 = [10^{-6}, 10^{-4}, \dots, 10^6]$<br>$C_2 = [10^{-6}, 10^{-4}, \dots, 10^6]$<br>$\mu = [2^{-5}, 2^{-4}, \dots, 2^5]$                  |
| H-ELM     | $C$ : Regularization parameter<br>$h_l$ : Number of hidden nodes                                                                                                                                   | $C = [10^{-6}, 10^{-4}, \dots, 10^6]$<br>$h_l = 5 : 10 : 205$                                                                               |
| F-BLS     | $C$ : Regularization parameter<br>$m$ : Number of feature groups<br>$p$ : Number of feature nodes in each groups<br>$q$ : Number of enhancement nodes                                              | $C = [10^{-6}, 10^{-4}, \dots, 10^6]$<br>$m = 1 : 2 : 21$<br>$p = 5 : 5 : 50$<br>$q = 5 : 10 : 105$                                         |
| IF-BLS    | $C$ : Regularization parameter<br>$m$ : Number of fuzzy groups<br>$p$ : Number of fuzzy nodes in each groups<br>$q$ : Number of enhancement nodes<br>$\mu$ : Intuitionistic fuzzy Kernel parameter | $C = [10^{-6}, 10^{-4}, \dots, 10^6]$<br>$m = 1 : 2 : 21$<br>$p = 5 : 5 : 50$<br>$q = 5 : 10 : 105$<br>$\mu = [2^{-5}, 2^{-4}, \dots, 2^5]$ |

Table S.II  
DESCRIPTION OF UCI DATASETS CHOSEN FOR EXPERIMENTS WITH ADDED GAUSSIAN NOISE.

| Dataset                      | Subject Area      | Win/Loss of the proposed IF-BLS model in 0% noise |
|------------------------------|-------------------|---------------------------------------------------|
| breast_cancer                | Life              | Loss                                              |
| conn_bench_sonar_mines_rocks | Physical          | Win                                               |
| hill_valley                  | Other (Synthetic) | Loss                                              |
| pittsburg_bridges_T_OR_D     | Civil Engineering | Win                                               |
| tic_tac_toe                  | Game              | Loss                                              |

performance at the noise level of 0% (indicating a loss for the proposed models) as per Table I of the main file of the paper. Additionally, we have chosen 2 datasets where the proposed F-BLS or IF-BLS model outperforms other models at the 0% noise level (indicating a win for the proposed models). For detailed information regarding the selected datasets, please refer to Table S.II.

### S.III. SENSITIVITY ANALYSIS OF THE PROPOSED F-BLS AND IF-BLS MODELS

In this section, we further analyze the dependency of the proposed models on the hyperparameters.

#### A. Performance Dependence on Feature Groups ( $m$ ), the Kernel Parameter ( $\mu$ ) and Regularization Parameter ( $C$ )

The testing accuracy of the proposed IF-BLS model for Alzheimer's disease diagnosis is depicted in Figures S.1, S.2, and S.3 for the CN\_VS\_AD, CN\_VS\_MCI, and MCI\_VS\_AD cases, respectively. The accuracy is evaluated by considering different numbers of feature groups ( $m$ ) while varying the Kernel parameter ( $\mu$ ) and regularization parameter ( $C$ ). One can observe that as the values of  $\mu$  and  $C$  increase, the accuracy also increases. However, beyond a certain point, the accuracy plateau is reached, indicating that the accuracy becomes less responsive to increases in  $\mu$  and  $C$ . Therefore, more attention is required to choose the hyperparameters.

Table S.III

THE STANDARD DEVIATIONS OF THE PROPOSED F-BLS AND IF-BLS MODELS ALONG WITH THE EXISTING MODELS, *i.e.*, BLS, ELM, NEUROFBLs, IF-TSVM, AND H-ELM ON UCI DATASETS.

| Dataset ↓   Model →            | BLS [2] | ELM [3] | NeuroFBLs [4] | IF-TSVM [5] | H-ELM [6] | F-BLS † | IF-BLS † |
|--------------------------------|---------|---------|---------------|-------------|-----------|---------|----------|
| acute_inflammation             | 0       | 0       | 0             | 6.8465      | 0         | 0       | 0        |
| acute_nephritis                | 0       | 0       | 0             | 49.3535     | 20.9165   | 0       | 0        |
| bank                           | 0.6268  | 0.5757  | 0.7048        | 0.5647      | 0.5977    | 0.6556  | 0.6945   |
| breast_cancer                  | 24.9547 | 34.1162 | 44.6249       | 44.6249     | 20.7893   | 27.5906 | 26.8828  |
| breast_cancer_wisc             | 3.9756  | 7.7412  | 5.2416        | 9.6852      | 6.6217    | 5.627   | 5.3499   |
| chess_krvkp                    | 2.4087  | 8.7903  | 3.6413        | 20.5579     | 12.3882   | 2.6204  | 2.4254   |
| conn_bench_sonar_mines_rocks   | 13.9054 | 5.6916  | 10.5182       | 25.3191     | 34.4077   | 11.3172 | 13.5518  |
| credit_approval                | 11.1132 | 10.506  | 10.5832       | 29.4322     | 11.9774   | 11.125  | 10.3423  |
| cylinder_bands                 | 3.4408  | 3.664   | 6.8956        | 17.9483     | 10.7841   | 3.2817  | 1.5525   |
| echocardiogram                 | 7.467   | 5.8108  | 3.6463        | 7.013       | 6.1721    | 7.2724  | 6.1265   |
| fertility                      | 10      | 9.6177  | 6.7082        | 10.3682     | 8.9443    | 8.2158  | 8.2158   |
| haberman_survival              | 7.3768  | 8.4751  | 8.4751        | 8.4751      | 8.0641    | 10.0681 | 8.5088   |
| hepatitis                      | 9.8374  | 9.5148  | 5.7705        | 14.1715     | 11.7642   | 9.5148  | 4.2059   |
| hill_valley                    | 6.8334  | 2.3404  | 4.4314        | 7.2928      | 8.8539    | 3.4346  | 4.279    |
| horse_colic                    | 4.9082  | 2.5627  | 2.9113        | 5.0495      | 1.4285    | 6.0478  | 2.5582   |
| mammographic                   | 2.4859  | 4.0207  | 5.5859        | 2.7999      | 2.928     | 4.8822  | 5.3901   |
| molec_biol_promoter            | 4.3409  | 6.4639  | 8.2564        | 26.2121     | 19.6765   | 3.7913  | 9.5415   |
| monks_1                        | 11.7835 | 8.4301  | 10.7869       | 5.6022      | 14.7166   | 7.6452  | 9.3321   |
| musk_1                         | 11.8581 | 4.8493  | 8.7957        | 36.0594     | 6.2829    | 7.25    | 7.7547   |
| oocytes_merluccius_nucleus_4d  | 2.5626  | 2.8977  | 3.7426        | 3.9544      | 4.1503    | 1.5154  | 2.2095   |
| oocytes_trisopterus_nucleus_2f | 4.6837  | 3.9279  | 2.6206        | 8.9408      | 3.7857    | 3.7965  | 2.3332   |
| pima                           | 2.8966  | 2.2956  | 4.2047        | 5.9529      | 4.9923    | 3.8226  | 1.5777   |
| pittsburg_bridges_T_OR_D       | 5.4205  | 11.5696 | 7.9461        | 13.9488     | 6.524     | 8.3581  | 5.9856   |
| spambase                       | 4.0884  | 5.5405  | 7.5672        | 53.9495     | 9.6543    | 2.8438  | 2.4424   |
| spect                          | 8.3745  | 3.5299  | 6.9325        | 14.0563     | 6.6172    | 2.7986  | 7.3802   |
| statlog_heart                  | 2.1114  | 3.5621  | 1.0143        | 2.6189      | 3.8401    | 2.8085  | 4.829    |
| tic_tac_toe                    | 1.2836  | 7.9105  | 13.1336       | 48.4173     | 25.876    | 1.7038  | 0.8768   |
| titanic                        | 15.5828 | 15.5828 | 13.6955       | 15.9056     | 15.75     | 15.5828 | 15.0381  |
| Average                        | 6.5829  | 6.7853  | 7.4441        | 17.6829     | 10.3037   | 6.1989  | 6.0494   |

### B. Performance Dependence on Number of Feature Nodes ( $p$ )

Moreover, to assess the impact of varying the number of feature nodes on the performance of the proposed F-BLS and IF-BLS models, Figure S.4 illustrates the relationship between the number of feature nodes and accuracy across five datasets: CN\_VS\_AD, CN\_VS\_MCI, MCI\_VS\_AD, breast\_cancer, and tic\_tac\_toe. The figure shows that increasing the number of feature nodes initially boosts accuracy. However, once a certain point is reached, increasing the number of feature nodes doesn't lead to much improvement in accuracy.

Specifically, for the F-BLS model, optimal accuracy is attained with just 25 nodes across all datasets. Conversely, the IF-BLS model exhibits varying patterns: for CN\_VS\_AD, tic\_tac\_toe, and MCI\_VS\_AD datasets, peak accuracy is also achieved with 25 nodes, whereas for CN\_VS\_MCI and breast\_cancer datasets, the optimal accuracy is achieved with 40 nodes. Consequently, a general recommendation emerges: fine-tuning the number of feature nodes from 25 onwards offers a promising avenue towards achieving optimal accuracy. However, it's important to note that the model's performance is dataset-dependent, necessitating careful hyperparameter tuning for each dataset to maximize accuracy.

Table S.IV

THE RANK OF THE PROPOSED F-BLS AND IF-BLS MODELS ALONG WITH THE EXISTING MODELS, *i.e.*, BLS, ELM, NEUROFBLs, IF-TSVM, AND H-ELM ON UCI DATASETS.

| Dataset ↓   Model →            | BLS [2] | ELM [3] | NeuroFBLs [4] | IF-TSVM [5] | H-ELM [6] | F-BLS † | IF-BLS † |
|--------------------------------|---------|---------|---------------|-------------|-----------|---------|----------|
| acute_inflammation             | 3.5     | 3.5     | 3.5           | 7           | 3.5       | 3.5     | 3.5      |
| acute_nephritis                | 3       | 3       | 3             | 7           | 6         | 3       | 3        |
| bank                           | 2       | 4.5     | 3             | 7           | 6         | 1       | 4.5      |
| breast_cancer                  | 6       | 7       | 4.5           | 4.5         | 1         | 3       | 2        |
| breast_cancer_wisc             | 3       | 5       | 1             | 7           | 6         | 4       | 2        |
| chess_krvkp                    | 2       | 5       | 6             | 7           | 4         | 3       | 1        |
| conn_bench_sonar_mines_rocks   | 3       | 6       | 5             | 7           | 2         | 4       | 1        |
| credit_approval                | 2       | 5       | 6             | 7           | 3         | 4       | 1        |
| cylinder_bands                 | 2       | 5       | 3             | 7           | 6         | 4       | 1        |
| echocardiogram                 | 4       | 5       | 6             | 7           | 2.5       | 2.5     | 1        |
| fertility                      | 4       | 5.5     | 1             | 7           | 5.5       | 2.5     | 2.5      |
| haberman_survival              | 6       | 4       | 4             | 4           | 2         | 7       | 1        |
| hepatitis                      | 3       | 5       | 1.5           | 7           | 6         | 4       | 1.5      |
| hill_valley                    | 1       | 5       | 4             | 7           | 6         | 2       | 3        |
| horse_colic                    | 3       | 5       | 6             | 7           | 2         | 4       | 1        |
| mammographic                   | 5       | 3       | 2             | 7           | 6         | 4       | 1        |
| molec_biol_promoter            | 3       | 5       | 6             | 7           | 4         | 2       | 1        |
| monks_1                        | 5       | 2       | 1             | 7           | 6         | 4       | 3        |
| musk_1                         | 4       | 5       | 6             | 7           | 1         | 3       | 2        |
| oocytes_merluccius_nucleus_4d  | 1       | 5       | 4             | 7           | 6         | 2       | 3        |
| oocytes_trisopterus_nucleus_2f | 1       | 3       | 4             | 7           | 6         | 2       | 5        |
| pima                           | 3       | 4       | 2             | 7           | 6         | 5       | 1        |
| pittsburg_bridges_T_OR_D       | 3       | 5       | 2             | 7           | 6         | 4       | 1        |
| spambase                       | 4       | 5       | 6             | 7           | 2         | 3       | 1        |
| spect                          | 2.5     | 4.5     | 4.5           | 7           | 6         | 2.5     | 1        |
| statlog_heart                  | 2.5     | 6       | 4.5           | 7           | 4.5       | 2.5     | 1        |
| tic_tac_toe                    | 1       | 4       | 5             | 7           | 6         | 2       | 3        |
| titanic                        | 4       | 4       | 2             | 7           | 6         | 4       | 1        |
| Average                        | 3.0893  | 4.6071  | 3.8036        | 6.8036      | 4.5357    | 3.2679  | 1.8929   |

Table S.V

THE BEST HYPERPARAMETERS OF THE PROPOSED F-BLS AND IF-BLS MODELS ALONG WITH THE EXISTING MODELS, *i.e.*, BLS, ELM, NEUROFBLs, IF-TSVM, AND H-ELM ON UCI DATASETS.

| Dataset ↓   Model →            | BLS [2]               | ELM [3]        | NeuroFBLs [4]            | IF-TSVM [5]                   | H-ELM [6]      | F-BLS †               | IF-BLS †                      |
|--------------------------------|-----------------------|----------------|--------------------------|-------------------------------|----------------|-----------------------|-------------------------------|
| Parameters                     | $(C, p, m, q)$        | $(C, h_1)$     | $(C, N_{fn}, N_{fg}, q)$ | $(C_1, C_2, \mu)$             | $(C, h_1)$     | $(C, p, m, q)$        | $(C, \mu, p, m, q)$           |
| acute_inflammation             | (0, 5, 9, 45)         | (0.000001, 15) | (0.000001, 5, 3, 5)      | (0.000001, 10000, 0.03125)    | (0.01, 25)     | (0.000001, 5, 5, 35)  | (100, 0.03125, 5, 3, 85)      |
| acute_nephritis                | (1, 5, 5, 35)         | (1, 45)        | (0.000001, 5, 1, 45)     | (0.000001, 10000, 0.03125)    | (0.0001, 85)   | (1, 5, 3, 105)        | (10000, 0.03125, 15, 9, 35)   |
| bank                           | (1000000, 25, 21, 85) | (10000, 195)   | (0.000001, 15, 15, 45)   | (0.000001, 1000000, 1)        | (0.01, 25)     | (1000000, 15, 15, 65) | (1000000, 0.5, 45, 19, 15)    |
| breast_cancer                  | (0, 15, 3, 105)       | (0.000001, 15) | (100, 5, 1, 5)           | (0.000001, 0.000001, 0.03125) | (0.000001, 35) | (0.000001, 40, 1, 55) | (1000000, 8, 5, 3, 75)        |
| breast_cancer_wisc             | (1, 25, 15, 85)       | (1, 155)       | (1, 30, 17, 55)          | (0.000001, 10000, 0.03125)    | (1, 45)        | (1, 35, 13, 75)       | (1000000, 1, 20, 21, 85)      |
| chess_krvkp                    | (0.01, 20, 3, 45)     | (10000, 165)   | (0.000001, 40, 21, 15)   | (1000000, 0.000001, 0.03125)  | (0.000001, 75) | (0.01, 40, 5, 15)     | (1000000, 0.03125, 30, 3, 75) |
| conn_bench_sonar_mines_rocks   | (0.01, 5, 3, 95)      | (10000, 165)   | (0.0001, 10, 17, 5)      | (10000, 0.000001, 0.03125)    | (0.0001, 135)  | (0.0001, 10, 1, 95)   | (1, 16, 50, 15, 105)          |
| credit_approval                | (0.01, 15, 1, 5)      | (10000, 45)    | (1, 5, 21, 15)           | (0.000001, 0.000001, 0.03125) | (0.01, 35)     | (0.01, 5, 15, 65)     | (100, 4, 10, 1, 85)           |
| cylinder_bands                 | (1, 25, 1, 85)        | (0.01, 125)    | (0.01, 15, 13, 95)       | (0.000001, 0.000001, 0.03125) | (0.01, 55)     | (1, 50, 13, 85)       | (100, 4, 5, 19, 65)           |
| echocardiogram                 | (1000000, 20, 1, 15)  | (0.01, 155)    | (1, 15, 3, 105)          | (0.000001, 1000000, 0.03125)  | (0.01, 125)    | (100, 10, 1, 105)     | (1000000, 8, 50, 19, 5)       |
| fertility                      | (100, 10, 1, 75)      | (0.000001, 55) | (1, 10, 9, 35)           | (0.000001, 0.000001, 0.03125) | (0.01, 115)    | (100, 45, 1, 85)      | (1000000, 1, 40, 17, 85)      |
| haberman_survival              | (1, 25, 21, 95)       | (0.000001, 5)  | (1, 5, 1, 5)             | (0.000001, 0.000001, 0.03125) | (0.0001, 55)   | (1000000, 45, 3, 5)   | (1000000, 16, 35, 1, 75)      |
| hepatitis                      | (100, 5, 3, 75)       | (0.01, 135)    | (0.0001, 45, 17, 55)     | (0.000001, 0.000001, 0.03125) | (0.01, 105)    | (1, 40, 19, 35)       | (10000, 8, 30, 5, 75)         |
| hill_valley                    | (0.01, 35, 9, 5)      | (0.01, 205)    | (1, 45, 21, 25)          | (10000, 1000000, 0.125)       | (0.01, 195)    | (1, 25, 19, 75)       | (1, 32, 50, 5, 55)            |
| horse_colic                    | (1, 35, 1, 55)        | (0.01, 175)    | (1, 5, 19, 95)           | (0.000001, 0.000001, 0.03125) | (1, 145)       | (1, 35, 7, 85)        | (1000000, 2, 50, 17, 15)      |
| mammographic                   | (10000, 10, 21, 45)   | (1000000, 75)  | (1, 15, 13, 15)          | (0.000001, 0.000001, 0.03125) | (0.0001, 5)    | (10000, 30, 1, 105)   | (1000000, 0.25, 10, 19, 85)   |
| molec_biol_promoter            | (0.01, 15, 15, 105)   | (0.01, 205)    | (0.0001, 25, 3, 45)      | (0.000001, 100, 0.03125)      | (0.0001, 35)   | (1, 20, 9, 5)         | (100, 8, 30, 7, 15)           |
| monks_1                        | (1000000, 10, 1, 95)  | (100, 205)     | (1, 50, 9, 75)           | (0.000001, 0.000001, 0.03125) | (0.01, 135)    | (1000000, 10, 1, 95)  | (1000000, 0.5, 45, 19, 85)    |
| musk_1                         | (0.01, 10, 3, 25)     | (0.0001, 205)  | (0.01, 35, 21, 5)        | (10000, 0.000001, 0.03125)    | (0.0001, 175)  | (0.01, 30, 13, 5)     | (10000, 16, 10, 17, 65)       |
| oocytes_merluccius_nucleus_4d  | (1, 35, 19, 55)       | (0.01, 175)    | (0.0001, 5, 21, 45)      | (1000000, 0.000001, 0.03125)  | (1, 165)       | (1, 30, 21, 65)       | (1000000, 0.0625, 40, 21, 55) |
| oocytes_trisopterus_nucleus_2f | (1000000, 30, 1, 25)  | (0.01, 205)    | (0.0001, 5, 19, 15)      | (1000000, 0.000001, 0.03125)  | (0.01, 145)    | (100, 40, 1, 75)      | (1000000, 0.5, 45, 19, 45)    |
| pima                           | (100, 30, 1, 25)      | (1000000, 105) | (0.01, 5, 9, 65)         | (0.000001, 0.000001, 0.03125) | (1, 55)        | (100, 20, 1, 5)       | (1000000, 1, 10, 9, 95)       |
| pittsburg_bridges_T_OR_D       | (1, 30, 21, 65)       | (0.0001, 15)   | (1, 40, 1, 75)           | (0.000001, 0.000001, 0.03125) | (0.0001, 125)  | (100, 30, 3, 15)      | (10000, 2, 40, 5, 95)         |
| spambase                       | (0.01, 30, 19, 65)    | (100, 175)     | (0.000001, 5, 19, 75)    | (0.000001, 0.000001, 0.03125) | (0.01, 75)     | (0.01, 10, 9, 55)     | (1, 16, 45, 19, 15)           |
| spect                          | (0.01, 5, 13, 55)     | (0.000001, 85) | (0.01, 45, 11, 55)       | (0.000001, 0.000001, 0.03125) | (1, 35)        | (1, 35, 5, 95)        | (100, 16, 25, 9, 25)          |
| statlog_heart                  | (1, 30, 9, 105)       | (0.01, 55)     | (1, 40, 15, 105)         | (0.000001, 0.000001, 0.03125) | (0.01, 55)     | (1, 50, 7, 105)       | (10000, 4, 25, 17, 55)        |
| tic_tac_toe                    | (1, 15, 21, 105)      | (10000, 205)   | (0.01, 35, 15, 95)       | (0.000001, 0.000001, 0.03125) | (0.000001, 85) | (1, 15, 21, 45)       | (10000, 2, 10, 21, 55)        |
| titanic                        | (10000, 10, 3, 65)    | (0.000001, 75) | (100, 5, 1, 55)          | (0.000001, 10000, 0.03125)    | (0.01, 5)      | (0.000001, 5, 1, 5)   | (1, 2, 15, 1, 65)             |

Table S.VI

THE STANDARD DEVIATIONS OF THE PROPOSED F-BLS AND IF-BLS MODELS ALONG WITH THE EXISTING MODELS, *i.e.*, BLS, ELM, NEUROFBLs, IF-TSVM, AND H-ELM ON UCI DATASET WITH VARYING LEVELS OF 5%, 10%, 15%, AND 20% GAUSSIAN NOISE.

| Dataset ↓   Model →          | Noise | BLS [2] | ELM [3] | NeuroFBLs [4] | IF-TSVM [5] | H-ELM [6] | F-BLS † | IF-BLS † |
|------------------------------|-------|---------|---------|---------------|-------------|-----------|---------|----------|
| breast_cancer                | 5%    | 26.0578 | 43.5886 | 44.6249       | 44.6249     | 21.5082   | 27.9532 | 23.9395  |
|                              | 10%   | 27.547  | 45.6714 | 44.6249       | 44.6249     | 20.109    | 27.6671 | 24.5976  |
|                              | 15%   | 27.0047 | 44.3655 | 43.9368       | 44.6249     | 27.4997   | 24.3874 | 21.4006  |
|                              | 20%   | 26.8794 | 42.3351 | 44.4418       | 44.6249     | 30.929    | 29.7448 | 23.919   |
| conn_bench_sonar_mines_rocks | 5%    | 9.8007  | 3.9134  | 7.7724        | 21.9294     | 31.0739   | 9.4446  | 8.9616   |
|                              | 10%   | 14.8713 | 12.8776 | 10.5432       | 24.0628     | 32.2191   | 7.7664  | 13.866   |
|                              | 15%   | 6.373   | 7.4754  | 13.0538       | 16.9866     | 13.0222   | 6.4177  | 8.7652   |
|                              | 20%   | 12.7508 | 5.4069  | 20.556        | 22.0657     | 26.5379   | 8.8397  | 15.2157  |
| hill_valley                  | 5%    | 0.4903  | 2.3907  | 3.1142        | 4.2855      | 6.9003    | 0.7357  | 3.366    |
|                              | 10%   | 2.3794  | 3.7976  | 0.4881        | 4.3653      | 4.1687    | 3.1585  | 2.092    |
|                              | 15%   | 1.961   | 2.4486  | 2.9256        | 1.5395      | 7.9389    | 1.9428  | 1.9166   |
|                              | 20%   | 2.419   | 2.1926  | 3.0069        | 2.0268      | 6.4379    | 2.4648  | 2.2579   |
| pittsburg_bridges_T_OR_D     | 5%    | 9.5855  | 13.9488 | 9.5615        | 13.9488     | 8.6481    | 8.4472  | 4.4237   |
|                              | 10%   | 8.3581  | 10.0785 | 7.9461        | 13.9488     | 13.9488   | 6.4957  | 5.6944   |
|                              | 15%   | 8.9271  | 11.9712 | 8.3734        | 13.9488     | 13.9488   | 4.5094  | 4.4639   |
|                              | 20%   | 7.4357  | 13.9488 | 5.6944        | 13.9488     | 13.4466   | 9.2637  | 5.5185   |
| tic_tac_toe                  | 5%    | 2.4968  | 20.0315 | 9.7246        | 48.3136     | 29.0264   | 2.1695  | 1.6115   |
|                              | 10%   | 2.0868  | 11.8785 | 10.5162       | 48.4173     | 24.1614   | 1.172   | 1.6671   |
|                              | 15%   | 2.3264  | 9.2264  | 13.3383       | 48.4173     | 37.2164   | 3.0788  | 1.5491   |
|                              | 20%   | 2.0997  | 14.1505 | 14.1961       | 48.4173     | 43.2215   | 3.362   | 1.9521   |
| Avg. Std. Dev.               |       | 10.0925 | 16.0849 | 15.92196      | 26.2561     | 20.5981   | 9.4511  | 8.8589   |

Table S.VII

THE HYPERPARAMETERS OF THE PROPOSED F-BLS AND IF-BLS MODELS ALONG WITH THE EXISTING MODELS, *i.e.*, BLS, ELM, NEUROFBLs, IF-TSVM, AND H-ELM ON UCI DATASET WITH VARYING LEVELS OF 5%, 10%, 15%, AND 20% GAUSSIAN NOISE.

| Dataset ↓   Model →          | Noise ↓ | BLS [2]              | ELM [3]        | NeuroFBLs [4]            | IF-TSVM [5]                   | H-ELM [6]       | F-BLS †               | IF-BLS †                       |
|------------------------------|---------|----------------------|----------------|--------------------------|-------------------------------|-----------------|-----------------------|--------------------------------|
| Parameters →                 |         | $(C, p, m, q)$       | $(C, h_l)$     | $(C, N_{fn}, N_{fg}, q)$ | $(C_1, C_2, \mu)$             | $(C, h_l)$      | $(C, p, m, q)$        | $(C, \mu, p, m, q)$            |
| breast_cancer                | 5%      | (0.0001, 10, 3, 105) | (0.000001, 5)  | (100, 5, 1, 5)           | (0.000001, 0.000001, 0.03125) | (0.000001, 125) | (0.0001, 10, 1, 95)   | (100, 16, 5, 1, 25)            |
|                              | 10%     | (0, 40, 1, 25)       | (0.000001, 5)  | (100, 5, 1, 5)           | (0.000001, 0.000001, 0.03125) | (0.000001, 5)   | (0.000001, 25, 1, 15) | (1000000, 8, 10, 1, 5)         |
|                              | 15%     | (0, 25, 1, 35)       | (0.0001, 5)    | (100, 20, 1, 25)         | (0.000001, 0.000001, 0.03125) | (0.0001, 95)    | (0.0001, 5, 3, 105)   | (1000000, 4, 5, 3, 85)         |
|                              | 20%     | (0, 15, 1, 65)       | (0.0001, 5)    | (100, 35, 17, 35)        | (0.000001, 0.000001, 0.03125) | (0.000001, 15)  | (0.0001, 15, 3, 5)    | (10000, 4, 15, 3, 45)          |
| conn_bench_sonar_mines_rocks | 5%      | (0.01, 10, 1, 95)    | (100, 115)     | (0.0001, 15, 13, 75)     | (10000, 0.000001, 0.03125)    | (0.000001, 175) | (0.01, 35, 3, 35)     | (1000000, 32, 50, 1, 105)      |
|                              | 10%     | (0.01, 5, 9, 95)     | (1000000, 145) | (0.000001, 10, 17, 95)   | (10000, 0.000001, 0.03125)    | (0.000001, 155) | (10000, 40, 9, 15)    | (100, 16, 35, 11, 5)           |
|                              | 15%     | (0.01, 5, 3, 55)     | (10000, 155)   | (0.0001, 20, 11, 95)     | (10000, 0.000001, 0.03125)    | (0.0001, 115)   | (0.0001, 50, 1, 45)   | (1, 32, 5, 19, 15)             |
|                              | 20%     | (0.01, 5, 17, 95)    | (10000, 75)    | (0.0001, 15, 11, 25)     | (10000, 0.000001, 0.03125)    | (0.0001, 195)   | (10000, 35, 21, 15)   | (10000, 32, 50, 1, 55)         |
| hill_valley                  | 5%      | (0.01, 20, 17, 55)   | (0.01, 175)    | (0.000001, 10, 17, 85)   | (100, 100, 16)                | (0.01, 195)     | (1, 35, 9, 85)        | (1000000, 0.0625, 25, 21, 75)  |
|                              | 10%     | (0.01, 50, 19, 55)   | (0.01, 205)    | (1, 15, 19, 15)          | (10000, 1000000, 0.03125)     | (0.01, 155)     | (0.01, 25, 17, 75)    | (1000000, 0.03125, 20, 19, 25) |
|                              | 15%     | (0.01, 30, 19, 25)   | (0.01, 205)    | (1, 35, 17, 95)          | (10000, 1000000, 0.03125)     | (0.01, 135)     | (0.01, 30, 11, 105)   | (1000000, 0.03125, 50, 19, 95) |
|                              | 20%     | (0.01, 45, 19, 95)   | (0.01, 195)    | (1, 35, 21, 45)          | (0.000001, 1000000, 0.03125)  | (0.01, 145)     | (0.01, 40, 21, 55)    | (1000000, 0.03125, 20, 15, 25) |
| pittsburg_bridges_T_OR_D     | 5%      | (100, 40, 1, 55)     | (0.000001, 5)  | (1, 30, 5, 55)           | (0.000001, 0.000001, 0.03125) | (0.01, 165)     | (100, 15, 3, 105)     | (100, 32, 20, 1, 85)           |
|                              | 10%     | (1000000, 45, 1, 25) | (1, 115)       | (1, 50, 1, 15)           | (0.000001, 0.000001, 0.03125) | (0.000001, 5)   | (100, 30, 9, 85)      | (100, 32, 40, 3, 85)           |
|                              | 15%     | (100, 5, 3, 65)      | (1000000, 35)  | (0.01, 15, 1, 5)         | (0.000001, 0.000001, 0.03125) | (0.000001, 5)   | (100, 20, 3, 45)      | (10000, 2, 45, 11, 15)         |
|                              | 20%     | (100, 45, 1, 25)     | (0.000001, 5)  | (1, 40, 7, 15)           | (0.000001, 0.000001, 0.03125) | (0.01, 145)     | (10000, 30, 21, 45)   | (10000, 2, 30, 5, 105)         |
| tic_tac_toe                  | 5%      | (1, 10, 21, 105)     | (1, 175)       | (0.000001, 15, 19, 25)   | (1000000, 0.000001, 0.03125)  | (0.0001, 25)    | (100, 10, 19, 75)     | (1000000, 1, 30, 21, 105)      |
|                              | 10%     | (1, 15, 21, 105)     | (1000000, 185) | (0.000001, 15, 19, 35)   | (0.000001, 0.000001, 0.03125) | (0.000001, 195) | (100, 35, 19, 105)    | (1000000, 1, 40, 21, 105)      |
|                              | 15%     | (1, 25, 21, 95)      | (100, 195)     | (0.01, 25, 13, 65)       | (0.000001, 0.000001, 0.03125) | (0.0001, 155)   | (1, 25, 21, 85)       | (1000000, 1, 25, 21, 75)       |
|                              | 20%     | (1, 25, 21, 105)     | (1, 185)       | (0.000001, 20, 15, 55)   | (0.000001, 0.000001, 0.03125) | (0.0001, 105)   | (100, 10, 19, 75)     | (1000000, 1, 10, 21, 75)       |

Table S.VIII

THE BEST HYPERPARAMETERS OF THE PROPOSED F-BLS AND IF-BLS MODELS ALONG WITH THE EXISTING MODELS, *i.e.*, BLS, ELM, NEUROFBLs, IF-TSVM, AND H-ELM ON ADNI DATASETS.

| Dataset ↓   Model → | BLS [2]           | ELM [3]      | NeuroFBLs [4]            | IF-TSVM [5]                   | H-ELM [6]   | F-BLS †               | IF-BLS †              |
|---------------------|-------------------|--------------|--------------------------|-------------------------------|-------------|-----------------------|-----------------------|
| Parameters          | $(C, p, m, q)$    | $(C, h_l)$   | $(C, N_{fn}, N_{fg}, q)$ | $(C_1, C_2, \mu)$             | $(C, h_l)$  | $(C, p, m, q)$        | $(C, \mu, p, m, q)$   |
| CN_VS_AD            | (1, 30, 11, 35)   | (100, 95)    | (0.01, 10, 9, 85)        | (0.000001, 1000000, 0.03125)  | (1, 105)    | (10000, 35, 3, 55)    | (100, 2, 15, 19, 95)  |
| CN_VS_MCI           | (100, 35, 19, 55) | (10000, 105) | (0.0001, 30, 3, 95)      | (0.000001, 0.000001, 0.03125) | (0.01, 115) | (10000, 4, 30, 7, 15) | (10000, 4, 30, 7, 15) |
| MCI_VS_AD           | (1, 40, 9, 45)    | (1, 125)     | (1, 10, 5, 85)           | (0.000001, 0.000001, 0.03125) | (0.01, 145) | (1, 35, 21, 45)       | (100, 16, 30, 3, 65)  |

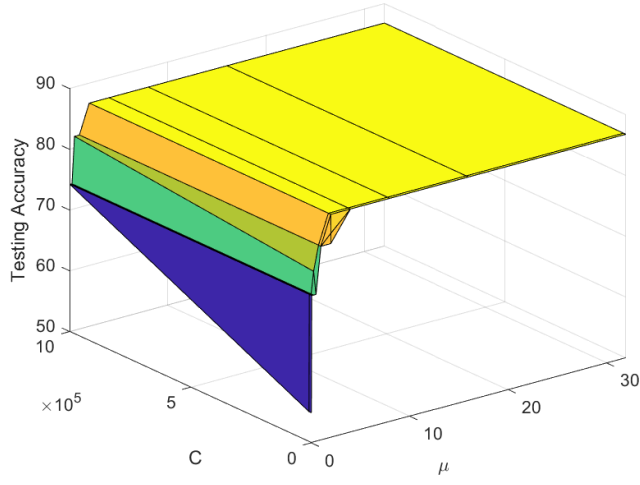(a)  $m = 3$ 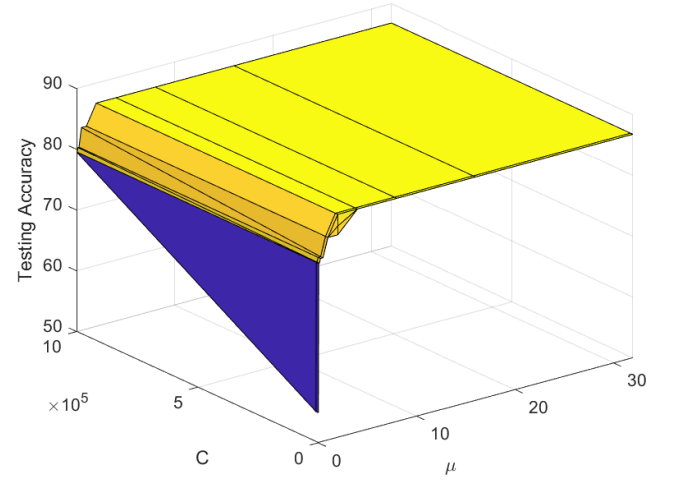(b)  $m = 9$ 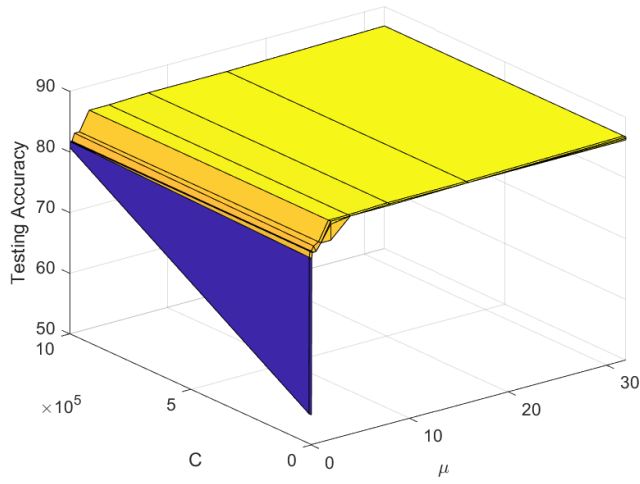(c)  $m = 15$ 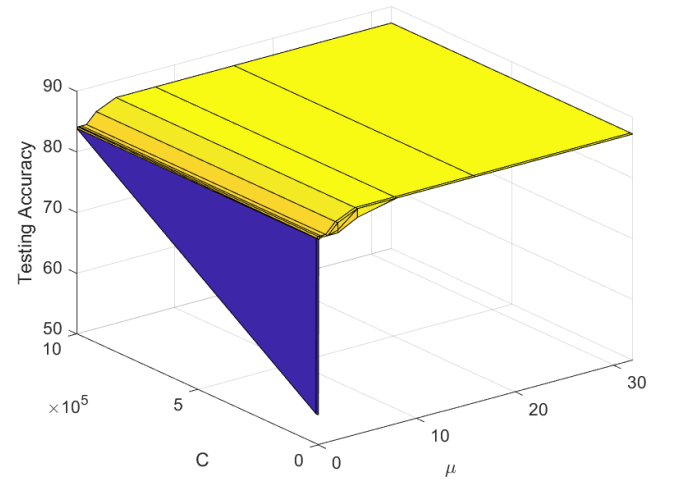(d)  $m = 21$ 

Figure S.1. Evaluation of the proposed IF-BLS model's testing accuracy on the CN\_VS\_AD case for Alzheimer's disease diagnosis, considering different numbers of feature groups ( $m$ ), while varying the Kernel parameter ( $\mu$ ) and regularization parameter ( $C$ ).

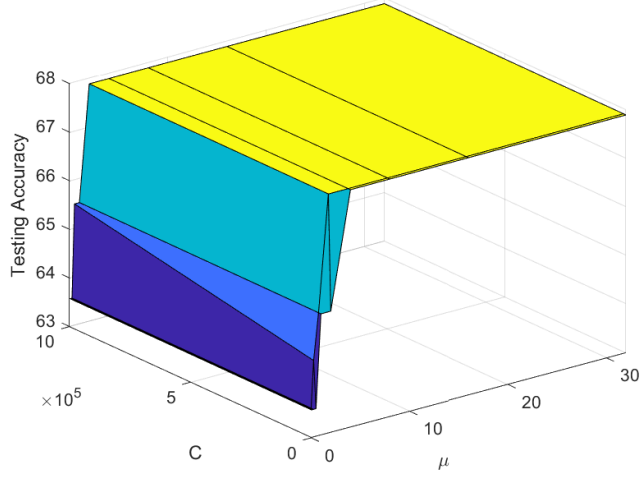(a)  $m = 3$ 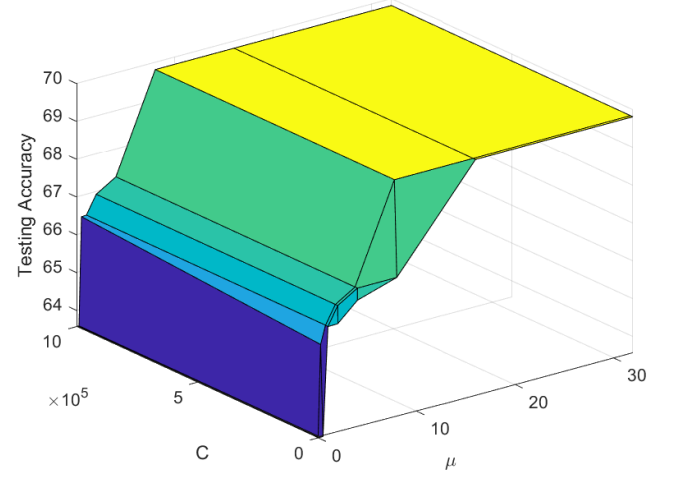(b)  $m = 9$ 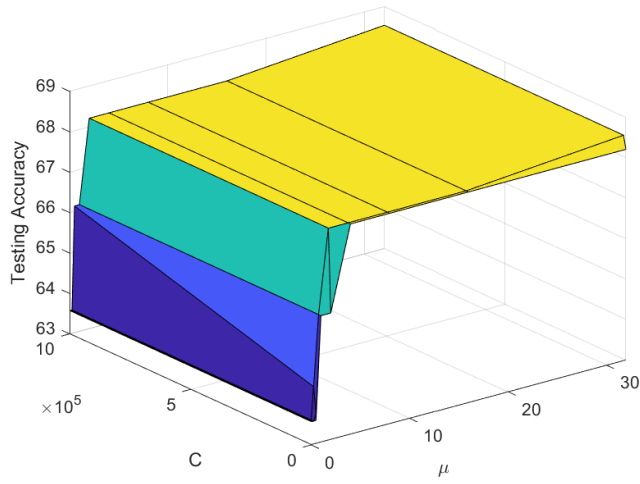(c)  $m = 15$ 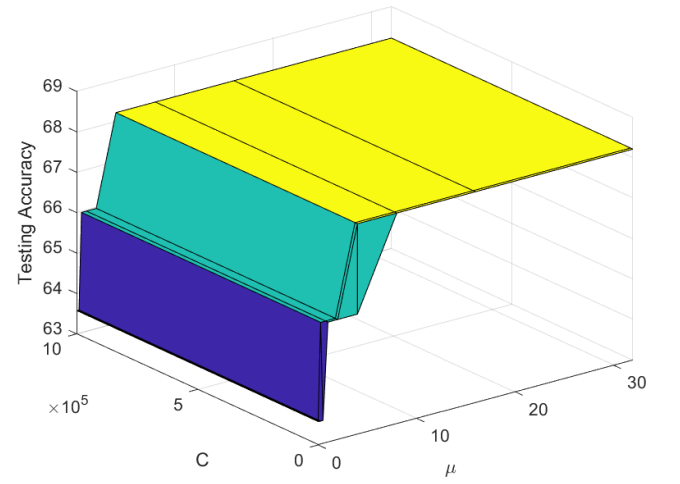(d)  $m = 21$ 

Figure S.2. Evaluation of the proposed IF-BLS model's testing accuracy on the CN\_VS\_MCI case for Alzheimer's disease diagnosis, considering different numbers of feature groups ( $m$ ), while varying the Kernel parameter ( $\mu$ ) and regularization parameter ( $C$ ).

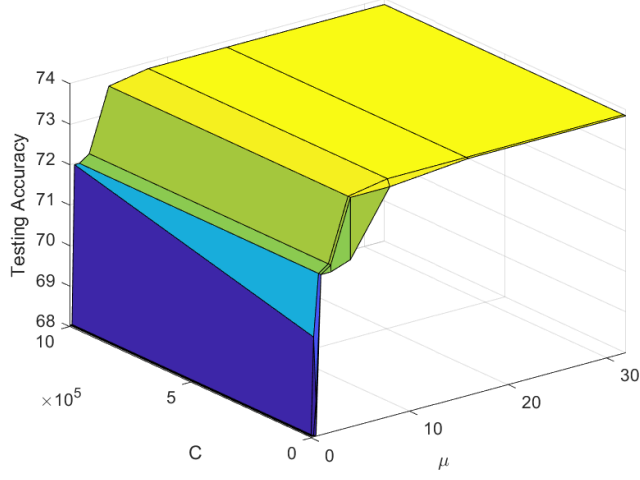(a)  $m = 3$ 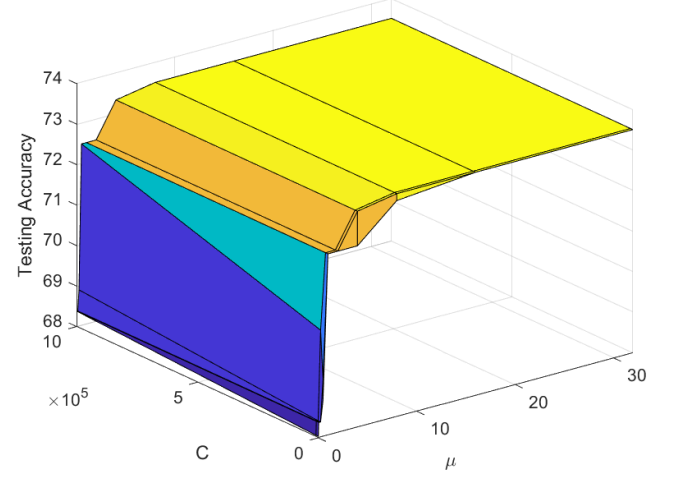(b)  $m = 9$ 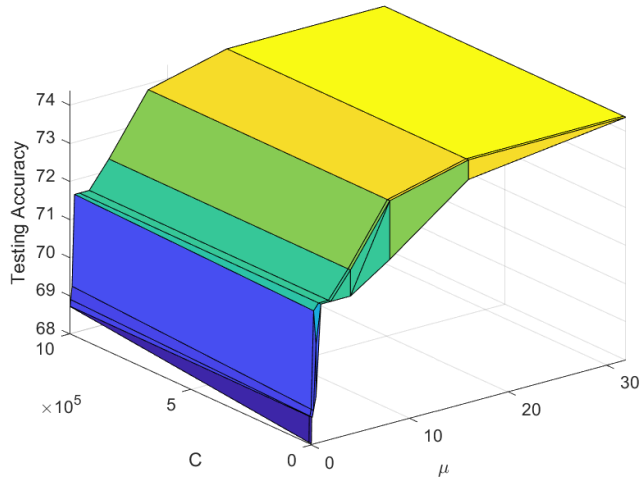(c)  $m = 15$ 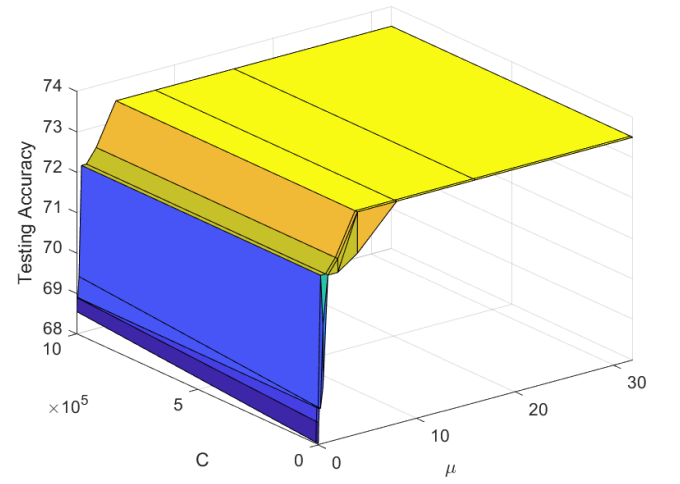(d)  $m = 21$ 

Figure S.3. Evaluation of the proposed IF-BLS model's testing accuracy on the MCI\_VS\_AD case for Alzheimer's disease diagnosis, considering different numbers of feature groups ( $m$ ), while varying the Kernel parameter ( $\mu$ ) and regularization parameter ( $C$ ).



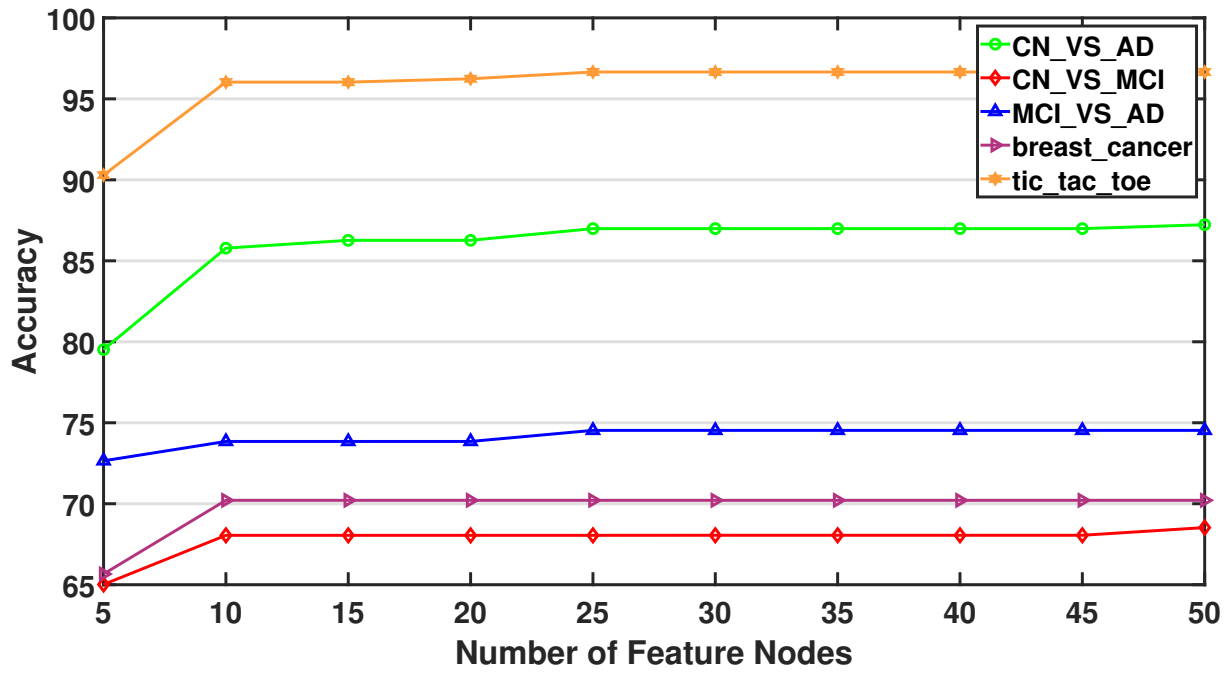

(a) F-BLS

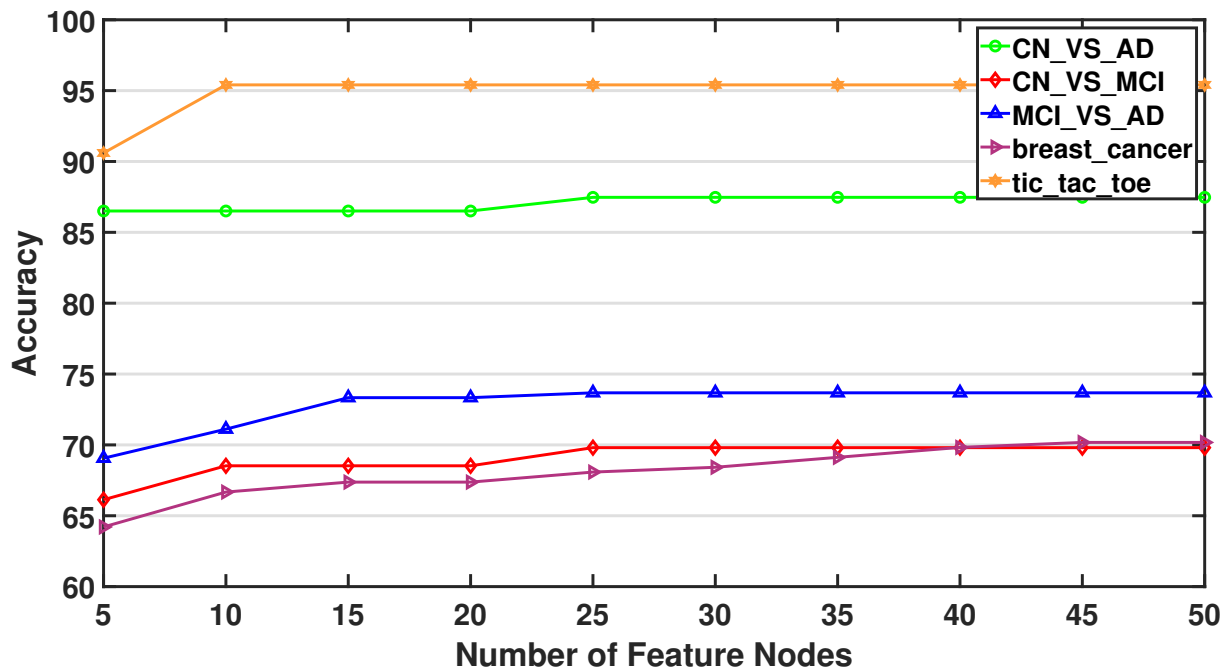

(b) IF-BLS

Figure S.4. Evaluation of the proposed F-BLS and IF-BLS models' testing accuracy while varying the number of feature nodes ( $p$ ).

## REFERENCES

- [1] M. Ha, C. Wang, and J. Chen, "The support vector machine based on intuitionistic fuzzy number and kernel function," *Soft Computing*, vol. 17, no. 4, pp. 635–641, 2013.
- [2] C. P. Chen and Z. Liu, "Broad learning system: An effective and efficient incremental learning system without the need for deep architecture," *IEEE Transactions on Neural Networks and Learning Systems*, vol. 29, no. 1, pp. 10–24, 2017.
- [3] G.-B. Huang, Q.-Y. Zhu, and C.-K. Siew, "Extreme learning machine: theory and applications," *Neurocomputing*, vol. 70, no. 1-3, pp. 489–501, 2006.
- [4] S. Feng and C. P. Chen, "Fuzzy broad learning system: A novel neuro-fuzzy model for regression and classification," *IEEE Transactions on Cybernetics*, vol. 50, no. 2, pp. 414–424, 2018.
- [5] S. Rezvani, X. Wang, and F. Pourpanah, "Intuitionistic fuzzy twin support vector machines," *IEEE Transactions on Fuzzy Systems*, vol. 27, no. 11, pp. 2140–2151, 2019.
- [6] J. Tang, C. Deng, and G.-B. Huang, "Extreme learning machine for multilayer perceptron," *IEEE Transactions on Neural Networks and Learning Systems*, vol. 27, no. 4, pp. 809–821, 2015.
